# Supplementary material for: Fine-Tuning is Fine, if Calibrated
Source: arXiv:2409.16223 source file (2024-10-13)
Supplement: Supplementary file 1 [file main_suppl.tex]

\documentclass[runningheads]{llncs}

% ---------------------------------------------------------------
% Include basic ECCV package
 
% TODO REVIEW: Insert your submission number below by replacing '*****'
% TODO FINAL: Comment out the following line for the camera-ready version
\usepackage[review,year=2024,ID=9855]{eccv}
% TODO FINAL: Un-comment the following line for the camera-ready version
%\usepackage{eccv}

% OPTIONAL: Un-comment the following line for a version which is easier to read
% on small portrait-orientation screens (e.g., mobile phones, or beside other windows)
%\usepackage[mobile]{eccv}

% ---------------------------------------------------------------
% Other packages

% Commonly used abbreviations (\eg, \ie, \etc, \cf, \etal, etc.)
\usepackage{eccvabbrv}

% Include other packages here, before hyperref.
\usepackage[dvipsnames]{xcolor}
\usepackage{graphicx}
\usepackage{booktabs}
\usepackage{amsmath}
\usepackage{amssymb}
\usepackage{mathtools}
\usepackage{wrapfig}
\usepackage{color, colortbl}
\definecolor{LightCyan}{rgb}{0.88,1,1}
\usepackage{pifont}
\usepackage{bbding}
\usepackage{makecell}
\usepackage{xspace}
\usepackage{subcaption}
\usepackage{caption}
\usepackage{bbm}
\usepackage{float}
\input{math_definition}
\usepackage{enumitem}
\usepackage{algorithm}
\usepackage{floatflt}
\usepackage{algpseudocode}
\usepackage{mathtools,tikz,caption}
\captionsetup{labelfont=sc,labelsep=period}
\DeclareRobustCommand\sampleline[1]{%
  \tikz\draw[#1] (0,0) (0,\the\dimexpr\fontdimen22\textfont2\relax)
  -- (2em,\the\dimexpr\fontdimen22\textfont2\relax);%
}

% The "axessiblity" package can be found at: https://ctan.org/pkg/axessibility?lang=en
\usepackage[accsupp]{axessibility}  % Improves PDF readability for those with disabilities.

% ---------------------------------------------------------------
% Hyperref package

% It is strongly recommended to use hyperref, especially for the review version.
% Please disable hyperref *only* if you encounter grave issues.
% hyperref with option pagebackref eases the reviewers' job, but should be disabled for the final version.
%
% If you comment hyperref and then uncomment it, you should delete
% main.aux before re-running LaTeX.
% (Or just hit 'q' on the first LaTeX run, let it finish, and you
%  should be clear).

% TODO FINAL: Comment out the following line for the camera-ready version
\usepackage[pagebackref,breaklinks,colorlinks,citecolor=eccvblue]{hyperref}
% TODO FINAL: Un-comment the following line for the camera-ready version
%\usepackage{hyperref}

% Support for ORCID icon
\usepackage{orcidlink}

\begin{document}

% ---------------------------------------------------------------
% TODO REVIEW: Replace with your title
%\title{Naive Fine-Tuning is Fine for Holistic Transfer} 
\title{Fine-Tuning is Fine with Partial Target Data}

% TODO REVIEW: If the paper title is too long for the running head, you can set
% an abbreviated paper title here. If not, comment out.
\titlerunning{Abbreviated paper title}

% TODO FINAL: Replace with your author list. 
% Include the authors' OCRID for the camera-ready version, if at all possible.
\author{First Author\inst{1}\orcidlink{0000-1111-2222-3333} \and
Second Author\inst{2,3}\orcidlink{1111-2222-3333-4444} \and
Third Author\inst{3}\orcidlink{2222--3333-4444-5555}}

% TODO FINAL: Replace with an abbreviated list of authors.
\authorrunning{F.~Author et al.}
% First names are abbreviated in the running head.
% If there are more than two authors, 'et al.' is used.

% TODO FINAL: Replace with your institution list.
\institute{Princeton University, Princeton NJ 08544, USA \and
Springer Heidelberg, Tiergartenstr.~17, 69121 Heidelberg, Germany
\email{lncs@springer.com}\\
\url{http://www.springer.com/gp/computer-science/lncs} \and
ABC Institute, Rupert-Karls-University Heidelberg, Heidelberg, Germany\\
\email{\{abc,lncs\}@uni-heidelberg.de}}

\maketitle

\input{arxiv/abstract}
\input{arxiv/intro}
\input{arxiv/background}
\input{arxiv/investigation}
\input{arxiv/method}
\input{arxiv/ablation}
\input{arxiv/why}
\input{arxiv/conclusion}
% \input{neurips2024/appendix}

% \clearpage\mbox{}Page \thepage\ of the manuscript.
% \clearpage\mbox{}Page \thepage\ of the manuscript.
% \clearpage\mbox{}Page \thepage\ of the manuscript.
% \clearpage\mbox{}Page \thepage\ of the manuscript.
% \clearpage\mbox{}Page \thepage\ of the manuscript. This is the last page.
% \par\vfill\par
% Now we have reached the maximum length of an ECCV \ECCVyear{} submission (excluding references).
% References should start immediately after the main text, but can continue past p.\ 14 if needed.
% \clearpage  % TODO REVIEW/FINAL: This \clearpage needs to be removed from both review and camera-ready versions.

% ---- Bibliography ----
%
% BibTeX users should specify bibliography style 'splncs04'.
% References will then be sorted and formatted in the correct style.
%
\bibliographystyle{splncs04}
\bibliography{main}

\end{document}
